# Supplementary material for: Loss Gradient Gaussian Width based Generalization and Optimization Guarantees
Source: arXiv:2406.07712 source file (2025-03-11)
Supplement: Supplementary file 1 [file app_empirical_arxiv.tex]

\begin{figure*}[h] 
\hspace*{-2mm}
\centering
 \subfigure[Top (sorted) gradient coordinate absolute values (linear scale).]{
  % [trim=left bottom right top, clip]
 \includegraphics[trim = 3mm 1mm 4mm 4mm, clip, width=0.28\textwidth]{figs/top_ut_linear_cifar.png}
 } % \vspace{-2mm}
 \hspace*{1mm}
  \subfigure[Top (sorted) gradient coordinate absolute values (log scale).]{
 \includegraphics[trim =3mm 1mm 4mm 4mm, clip, width=0.28\textwidth]{figs/top_ut_log_cifar.png}
 } % \vspace{-2mm}
  \vspace{-2mm}
 \hspace*{1mm}
 \subfigure[All (sorted) gradient coordinate absolute values (linear scale).]{
 \includegraphics[trim =3mm 1mm 4mm 4mm, clip, width=0.28\textwidth]{figs/all_ut_linear_cifar.png}
 } % \vspace{-2mm}
\caption{Sorted components of gradients for mini-batch SGD over 100 epochs on CIFAR-10, batch size 128, learning rate 0.01, averaged over 5 runs. Model is a 4-hidden-layer ReLU network with 256 nodes each layer, with around 1,055,000 parameters. Y-axis is the absolute value of sorted gradient coordinates, i.e., $|\mu_{t,(j)}|$, X-axis is sorted in increasing order.}
\vspace*{-3mm}
\label{fig:cifar_eva_app}
\end{figure*}

% \begin{figure*}[t] 
% \centering
%  \subfigure[SGD]{
%   % [trim=left bottom right top, clip]
%  \includegraphics[trim = 3mm 1mm 4mm 4mm, clip, width=0.30\textwidth]{figs/eva_mnist_sgd.png}
%  } % \vspace{-2mm}
%   \subfigure[DP-SGD, $\sigma = 1.0$]{
%  \includegraphics[trim =3mm 1mm 4mm 4mm, clip, width=0.30\textwidth]{figs/eva_mnist_dpsgd_no1.png}
%  } % \vspace{-2mm}
%  \subfigure[DP-SGD, $\sigma = 2.0$]{
%   % [trim=left bottom right top, clip]
%  \includegraphics[trim = 3mm 1mm 4mm 4mm, clip, width=0.30\textwidth]{figs/eva_mnist_dpsgd_no2.png}
%  }
%  \vspace{-3mm} 
% \caption[]{Top 500 eigen-value spectrum of the gradient second moment matrix along the training trajectory of SGD, DP-SGD with noise variance $\sigma=1, 2$. Dataset: MNIST; model: 2-layer ReLU with 128 nodes each layer. The network has roughly 130,000 parameters and is trained on MNIST dataset. The Y-axis is the eigenvalue and X-axis is order of eigenvalues from largest to smallest.}
% \vspace{-4mm}
% \label{fig:mnist_eva_app}
% \end{figure*}
%\vspace{-2mm}

\begin{figure*}[h]
\hspace*{-2mm}
\centering
 \subfigure[Top (sorted) gradient coordinate absolute values (linear scale).]{
  % [trim=left bottom right top, clip]
 \includegraphics[trim = 3mm 1mm 4mm 4mm, clip, width=0.28\textwidth]{figs/top_ut_linear.png}
 } % \vspace{-2mm}
 \hspace*{1mm}
  \subfigure[Top (sorted) gradient coordinate absolute values (log scale).]{
 \includegraphics[trim =3mm 1mm 4mm 4mm, clip, 
 width=0.28\textwidth]{figs/top_ut_log.png}
 } % \vspace{-2mm}
 \hspace*{1mm}
 \subfigure[All (sorted) gradient coordinate absolute values, sorted (linear scale).]{
 \includegraphics[trim =3mm 1mm 4mm 4mm, clip, width=0.28\textwidth]{figs/all_ut_linear.png}
 } 
 \vspace{-2mm}
\caption{Sorted components of gradients for mini-batch SGD over 100 epochs on MNIST, batch size 128, learning rate 0.01, averaged over 5 runs. Model is a 2-hidden-layer ReLU network with 128 nodes each layer, with around 120,000 parameters. Y-axis is the absolute value of sorted gradient coordinates, i.e., $|\mu_{t,(j)}|$, X-axis is sorted in increasing order. }
%for $j$-th coordinates. X-axis is order of $|\mu_t(j)|$. 
%\abcomment{legend has typo; need to explain y-axis; over how many iterations}
\vspace*{-1mm}
\label{fig:mnist_eva_app}
\end{figure*}
